# Supplementary material for: Continuous Control of Editing Models via Adaptive-Origin Guidance
Source: arXiv:2602.03826 source file (2026-02-03)
Supplement: Supplementary file 1 [file 6_appendix.tex]

\subsection{Analysis}
\paragraph{REC token}
what is p(z|Ci,REC)?
it is delta function over Ci. 

\paragraph{cfg with REC}
division and multiplication of gaussians.

\paragraph{our method}

Multiplications of gaussians over-time.
